# Supplementary material for: DEEP-IoT: Downlink-Enhanced Efficient-Power Internet of Things
Source: arXiv:2403.00321 source file (2024-11-15)
Supplement: Supplementary file 1 [file AppendixB.tex]

From the definition of the index in \eqref{eq:defidx}, we have
\begin{eqnarray}
&&\hspace{-0.5cm}\frac{\partial \mu_*(\bm{s}_{\ell},a_{\ell})}{\partial a_{\ell}} 
= \frac{\partial q_*(\bm{s}_{\ell},a_{\ell})}{\partial a_{\ell}} \\
&&\hspace{-0.5cm}
= \int_{h^\prime_{\ell},\widetilde{h}^\prime_{\ell}}\frac{\partial v_*\left(\bm{s}^\prime_{\ell}=\left[\text{E}^\prime_{\ell},h^\prime_{\ell},\widetilde{h}^\prime_{\ell}\right]\right)}{\partial a_{\ell}}\Pr(h^\prime_{\ell},\widetilde{h}^\prime_{\ell})d h^\prime_{\ell}d\widetilde{h}^\prime_{\ell} \nonumber\\
&&\hspace{-0.5cm}
=\mathbb{E}_{h^\prime_{\ell},\widetilde{h}^\prime_{\ell}}\left[\frac{\partial v_*\left(\bm{s}^\prime_{\ell}\right)}{\partial \text{E}^\prime_{\ell}}\frac{\partial \text{E}^\prime_{\ell}}{\partial a_{\ell}} \right].\nonumber
\end{eqnarray}

From Lemma \ref{thm:lem1}, we have $\frac{\partial v_*\left(\bm{s}^\prime_{\ell}\right)}{\partial \text{E}^\prime_{\ell}}\geq 0$. Furthermore,
\begin{eqnarray*}
&&\hspace{-0.5cm}
\frac{\partial \text{E}^\prime_{\ell}}{\partial a_{\ell}}=
-\frac{\partial \text{ET}^\prime_{\ell}}{\partial a_{\ell}} \\
&&\hspace{-0.5cm}
=
-\frac{\partial}{\partial a_{\ell}} \min\left\{P_{\max},10^{\frac{1}{10}\eta^*_{\text{dB}}\left(\widetilde{h}_{\ell},a_{\ell}\right)}\frac{N_0}{\alpha_{\ell}|h_{\ell}|^2}\right\}T_{\text{OFDM}}QG,
\end{eqnarray*}
where
\begin{eqnarray*}
&&\hspace{-0.65cm}
\frac{\partial \eta^*_{\text{dB}}\!\left(\widetilde{h}_{\ell},a_{\ell}\right)}{\partial a_{\ell}}\!=\!
-\!\left[\frac{1}{ \exp\!\left(u_0\widetilde{\eta}_{\text{dB}}\!+\!u_1 a_{\ell}\!+\!u_2\widetilde{\eta}_{\text{dB}} a_{\ell} \!+\! u_3\right) \!+\! u_4}\right]^2 \\
&&\hspace{0.7cm}
\exp\!\left(u_0\widetilde{\eta}_{\text{dB}}+u_1 a_{\ell}+u_2\widetilde{\eta}_{\text{dB}} a_{\ell} + u_3\right)(u_1+u_2\widetilde{\eta}_{\text{dB}}).
\end{eqnarray*}

Therefore, the positivity or negativity of $\frac{\partial \text{E}^\prime_{\ell}}{\partial a_{\ell}}$ and $\frac{\partial \mu_*(\bm{s}_{\ell},a_{\ell})}{\partial a_{\ell}}$  depends on $u_1+u_2\widetilde{\eta}_{\text{dB}}$. 
Since $u_2>0$, we have the following results: when $\widetilde{\eta}_{\text{dB}}\geq-\frac{u_1}{u_2}$, $\frac{\partial \mu_*(\bm{s}_{\ell},a_{\ell})}{\partial a_{\ell}}\geq 0$; when $\widetilde{\eta}_{\text{dB}}<-\frac{u_1}{u_2}$, $\frac{\partial \mu_*(\bm{s}_{\ell},a_{\ell})}{\partial a_{\ell}}\leq 0$. Lemma \ref{thm:lem2} is proved.
