# Supplementary material for: DEEP-IoT: Downlink-Enhanced Efficient-Power Internet of Things
Source: arXiv:2403.00321 source file (2024-11-15)
Supplement: Supplementary file 2 [file AppendixC.tex]

The index of an action $a_{\ell}>0$ can be written as:
\begin{eqnarray}\label{eq:APPC1}
&&\hspace{-0.5cm}
\mu_*(\bm{s}_{\ell},a_{\ell}) = q_*(\bm{s}_{\ell},a_{\ell}) - q_*(\bm{s}_{\ell},0) \\
&&\hspace{-0.5cm}
=\mathbb{E}_{h^\prime_{\ell},\widetilde{h}^\prime_{\ell}}\left[
v_*\left(\left[\text{E}^\prime_{\ell}(a_{\ell}),h^\prime_{\ell},\widetilde{h}^\prime_{\ell}\right]\right)-v_*\left(\left[\text{E}^\prime_{\ell}(0),h^\prime_{\ell},\widetilde{h}^\prime_{\ell}\right]\right)
\right],\nonumber
\end{eqnarray}
where
\begin{eqnarray*}
\text{E}^\prime_{\ell}(a_{\ell})
\hspace{-0.2cm}&=&\hspace{-0.2cm}
\text{E}_{\ell}-\text{ET}_{\ell}(h_{\ell},\widetilde{h}_{\ell},a_{\ell}) - \text{ER}_{\ell},
\\
\text{E}^\prime_{\ell}(0)
\hspace{-0.2cm}&=&\hspace{-0.2cm}
\text{E}_{\ell}-\text{ET}_{\ell}(h_{\ell},\widetilde{h}_{\ell},0) - \text{ES}_{\ell}.
\end{eqnarray*}

Since $v_*(\bm{s}_{\ell})$ is monotonic in $\text{E}_{\ell}$, the positive or negative of $\mu_*(\bm{s}_{\ell},a_{\ell})$ depends on the positive or negative of
\begin{eqnarray}\label{eq:APPC2}
&&\hspace{-0.65cm}
\text{E}^\prime_{\ell}(a_{\ell})-\text{E}^\prime_{\ell}(0)
\\
&&\hspace{-0.65cm}
=\text{ET}_{\ell}(h_{\ell},\widetilde{h}_{\ell},0)-\text{ET}_{\ell}(h_{\ell},\widetilde{h}_{\ell},a_{\ell})+\text{ES}_{\ell}-\text{ER}_{\ell}
\nonumber\\
&&\hspace{-0.65cm}
=\min\Big\{P_{\max},10^{\frac{1}{10}\eta^*_{\text{dB}}(0)}\frac{N_0}{\alpha_{\ell}|h_{\ell}|^2}\Big\}T_{\text{OFDM}}QG - \min\Big\{P_{\max},
\nonumber\\
&&\hspace{-0.65cm}
10^{\frac{1}{10}\eta^*_{\text{dB}}\left(\widetilde{h}_{\ell},a_{\ell}\right)}\frac{N_0}{\alpha_{\ell}|h_{\ell}|^2}\Big\}T_{\text{OFDM}}QG
\!-\! (P_r\!\!-\!\!P_s)T_{\text{OFDM}}Q(G\!-\!1). \nonumber
\end{eqnarray}

Defining $P^{\prime}_{\max}\triangleq\frac{\alpha_{\ell}|h_{\ell}|^2}{N_0}P_{\max}$ and multiplying the both sides of \eqref{eq:APPC2} by $\frac{\alpha_{\ell}|h_{\ell}|^2}{N_0T_{\text{OFDM}}QG}$, we have
\begin{eqnarray}\label{eq:APPC3}
&&\hspace{-0.65cm}
H\triangleq\frac{\alpha_{\ell}|h_{\ell}|^2}{N_0T_{\text{OFDM}}QG}\left[\text{E}^\prime_{\ell}(a_{\ell})-\text{E}^\prime_{\ell}(0)\right]
\\
&&\hspace{-0.65cm}
=\min\Big\{P^\prime_{\max},10^{\frac{1}{10}\eta^*_{\text{dB}}(0)}\Big\} - \min\Big\{P^\prime_{\max},10^{\frac{1}{10}\eta^*_{\text{dB}}\left(\widetilde{h}_{\ell},a_{\ell}\right)}\Big\}
\nonumber\\
&&\hspace{-0.3cm}
- \frac{G-1}{G}(P_r-P_s)\frac{\alpha_{\ell}|h_{\ell}|^2}{N_0}. \nonumber
\end{eqnarray}

To further simplify \eqref{eq:APPC3}, we have to compare $P^\prime_{\max}$, $10^{\frac{1}{10}\eta^*_{\text{dB}}(0)}$, and $10^{\frac{1}{10}\eta^*_{\text{dB}}\left(\widetilde{h}_{\ell},a_{\ell}\right)}$. 

Case I: $10^{\frac{1}{10}\eta^*_{\text{dB}}(0)}\geq P^\prime_{\max}$ and $10^{\frac{1}{10}\eta^*_{\text{dB}}\left(\widetilde{h}_{\ell},a_{\ell}\right)}\geq  P^\prime_{\max}$. In this case,
\begin{equation*}
H= P^\prime_{\max} - P^\prime_{\max} - \frac{G-1}{G}(P_r-P_s)\frac{\alpha_{\ell}|h_{\ell}|^2}{N_0} < 0.
\end{equation*}
Therefore, $\text{E}^\prime_{\ell}(a_{\ell})<\text{E}^\prime_{\ell}(0)$ and $\mu_*(\bm{s}_{\ell},a_{\ell})<0$.

Case II: $10^{\frac{1}{10}\eta^*_{\text{dB}}(0)}< P^\prime_{\max}$ and $10^{\frac{1}{10}\eta^*_{\text{dB}}\left(\widetilde{h}_{\ell},a_{\ell}\right)}\geq  P^\prime_{\max}$. In this case,
\begin{equation*}
H= 10^{\frac{1}{10}\eta^*_{\text{dB}}(0)} - P^\prime_{\max} - \frac{G-1}{G}(P_r-P_s)\frac{\alpha_{\ell}|h_{\ell}|^2}{N_0} < 0.
\end{equation*}
Therefore, we also have $\text{E}^\prime_{\ell}(a_{\ell})<\text{E}^\prime_{\ell}(0)$ and $\mu_*(\bm{s}_{\ell},a_{\ell})<0$.

In actuality, comparing $P^\prime_{\max}$ and $10^{\frac{1}{10}\eta^*_{\text{dB}}(0)}$ is essentially comparing $10\lg\frac{\alpha_{\ell}|h_{\ell}|^2}{N_0}P_{\max}$ and $\eta^*_{\text{dB}}(0)$, where the former is the maximum UL received SNR at the AP when the IoT device uses the maximum power $P_{\max}$ to transmit. To simply notation, we define $\eta^{\text{max}}_{\text{dB}}\triangleq 10\lg\frac{\alpha_{\ell}|h_{\ell}|^2}{N_0}P_{\max}$. Similarly, comparing $P^\prime_{\max}$ and $10^{\frac{1}{10}\eta^*_{\text{dB}}\left(\widetilde{h}_{\ell},a_{\ell}\right)}$ is essentially comparing $\eta^{\text{max}}_{\text{dB}}$ and $\eta^*_{\text{dB}}\left(\widetilde{h}_{\ell},a_{\ell}\right)$.

In the first two cases, we have $\eta^{\text{max}}_{\text{dB}}\leq\eta^*_{\text{dB}}\left(\widetilde{h}_{\ell},a_{\ell}\right)$. This means that DEEP-IoT requires a forward SNR $\eta^*_{\text{dB}}\left(\widetilde{h}_{\ell},a_{\ell}\right)$ even larger than the UL link can possibly provide with the largest transmit power. As a result, it is better not to use feedback coding, but using traditional forward coding instead. That is why we have $\mu_*(\bm{s}_{\ell},a_{\ell})<0$.

Case III: $10^{\frac{1}{10}\eta^*_{\text{dB}}(0)}\geq P^\prime_{\max}$ and $10^{\frac{1}{10}\eta^*_{\text{dB}}\left(\widetilde{h}_{\ell},a_{\ell}\right)}<  P^\prime_{\max}$. In this case,
\begin{equation*}
H= P^\prime_{\max} - 10^{\frac{1}{10}\eta^*_{\text{dB}}\left(\widetilde{h}_{\ell},a_{\ell}\right)} - \frac{G-1}{G}(P_r-P_s)\frac{\alpha_{\ell}|h_{\ell}|^2}{N_0}
\end{equation*}
can be either positive or negative. However, from the conditions, we know that $\eta^*_{\text{dB}}\left(\widetilde{h}_{\ell},a_{\ell}\right)<\eta^{\text{max}}_{\text{dB}}\leq\eta^*_{\text{dB}}(0)$. This suggests that the target BLER can be achieved by only feedback coding, but not the traditional forward coding. Thus, although the sign of $\mu_*(\bm{s}_{\ell},a_{\ell})<0$ is undetermined, we should choose $a_{\ell}$ in case III.

Case IV: $10^{\frac{1}{10}\eta^*_{\text{dB}}(0)}< P^\prime_{\max}$ and $10^{\frac{1}{10}\eta^*_{\text{dB}}\left(\widetilde{h}_{\ell},a_{\ell}\right)}<  P^\prime_{\max}$. In this case,
\begin{equation*}
H= 10^{\frac{1}{10}\eta^*_{\text{dB}}(0)} - 10^{\frac{1}{10}\eta^*_{\text{dB}}\left(\widetilde{h}_{\ell},a_{\ell}\right)} - \frac{G-1}{G}(P_r-P_s)\frac{\alpha_{\ell}|h_{\ell}|^2}{N_0},
\end{equation*}
the sign of which is undetermined. In addition, both $\eta^*_{\text{dB}}\left(\widetilde{h}_{\ell},a_{\ell}\right)$ and $\eta^*_{\text{dB}}(0)$ are smaller than $\eta^{\text{max}}_{\text{dB}}$, the target BLER can be achieved by both feedback and forward coding.
